# Supplementary material for: Understanding the Nonlinear Dynamics of Driven Particles in Supercooled Liquids in Terms of an Effective Temperature
Source: arXiv:1511.05828 source file (2015-11-26)
Supplement: Supplementary file 1 [file JCPSupp-2.pdf]

# Supplemental Material to "Understanding the Nonlinear Dynamics of Driven Particles in Supercooled Liquids in Terms of an Effective Temperature"

Carsten F. E. Schroer[1,2,a] and Andreas Heuer[1,2,b]

[1] *Westfälische Wilhelms-Universität Münster, Institut für physikalische Chemie, Corrensstraße 28/30, 48149 Münster, Germany*

[2] *NRW Graduate School of Chemistry, Wilhelm-Klemm-Straße 10, 48149 Münster, Germany*

(Dated: 18 November 2015)

[a] Electronic mail: c.schroer@uni-muenster.de

[b] Electronic mail: andheuer@uni-muenster.de

## MICRORHEOLOGY AND THERMOSTAT PROPERTIES

The results which are presented in the main article have been obtained from simulations of a $NVT$ ensemble. To guarantee isothermal conditions the bath particles, i.e., all particles except of the tracer particle, have been coupled to a chain of five Nosé-Hoover-thermostats[1–3]. The virtual mass $Q_0$ of the central thermostat, which is directly coupled to the bath particles, has been chosen as $Q_0 = 2Nk_\mathrm{B}T$, the chain thermostats' masses as $Q_i = 2k_\mathrm{B}T$. For an undriven system, this parameters offer a reasonable distribution of kinetic energies $\epsilon_\mathrm{kin}$.

In the article, we study the system under the condition that the tracer particle is pulled by an external force. Due to the forcing, the particle is constantly accelerated along the force field's direction and transfers the additional kinetic energy via collisions to the bath particles, thereby approaching a stationary state. In the limit of small forces, this additional kinetic energy will be small. It is therefore to be reasonable to assume that it can be quickly dissipated among the bath particles and afterwards be removed from the system by the thermostat. For high forces, especially in nonlinear response regime, it is *a priori* unclear, whether the thermostat is still able to conserve the average temperature. This is of particular

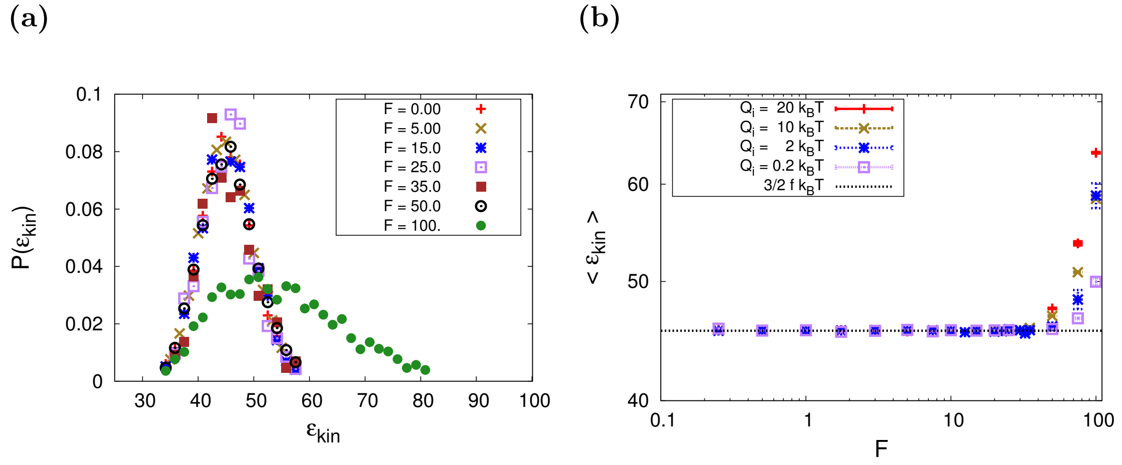


FIG. 1: **Thermostat properties in the non-equilibrium situation.** (a) Distribution of the kinetic energy of the bath particles at temperature $T = 0.475$ and different forces $F$. (b) Average kinetic energy of the system $\langle\epsilon_\mathrm{kin}\rangle$ at $T = 0.475$ for different forces $F$ and virtual masses $Q_i$ of the Nosé-Hoover-thermostat. The dashed line corresponds to the theoretically expected value $\langle\epsilon_\mathrm{kin}\rangle = \frac{1}{2}fk_\mathrm{B}T$, where $f$ denotes the degrees of freedom of the system.

importance, since the Potential Energy Landscape approach restricts us to simulations with a small number of particles.

To study this we have computed the distribution of the kinetic energy $\epsilon_{\text{kin}}$ of the bath particles at $T = 0.475$ for a broad range of forces. As one can observe in Fig. 1(a), the distribution of $\epsilon_{\text{kin}}$ is still in agreement with the distribution of the undriven system, even at large forces. Only at extremely large field strength ($F \geq 50$) the distribution starts to differ in both, shape and average value. Please consider that for the given temperature, the onset of nonlinearity can be expected for force strengths $F \approx 3$. Thus, even in the regime of strong nonlinear response, we observe that the system is not heated up.

Furthermore, it might be arguable, whether the particular choice of $Q_i$ is of crucial importance for the system's thermal behavior. We therefore have conducted additional simulations of the system with different virtual thermostat masses $Q_i = 0.2\ k_{\text{B}}T, 10\ k_{\text{B}}T, 20\ k_{\text{B}}T$, and $Q_0 = NQ_i$, respectively. The average values $\langle\epsilon_{\text{kin}}\rangle$ of the kinetic energy for different forces are shown in Fig. 1(b). For all virtual masses one does not observe an increase of the kinetic energy up to $F \approx 50$. For forces lower than that there is additionally no relevant dependence of $\langle\epsilon_{\text{kin}}\rangle$ on the chosen virtual mass; both graphs recover the expectation value predicted by the kinetic gas theory. Only for $F \geq 50$, where the system displays an unphysical behavior anyway, a dependence on the chosen virtual masses can be observed. Therefore, for the range of forces we are discussing in our main article ($0 \leq F \leq 25$), the chosen parameters for the thermostat are sufficient to guarantee isothermal conditions.

## POTENTIAL ENERGY LANDSCAPE MINIMA UNDER APPLICATION OF AN EXTERNAL FORCE

In the main article we study the dynamics of a fragile glass-former in terms of escape events out of minima of its Potential Energy Landscape (PEL). The energy minima are computed by varying the coordinates $\vec{r}_1, \vec{r}_2, ..., \vec{r}_N$ of the $N$ particles of the system in such a way, that the potential energy function

$$V_0(\vec{r}_1, \vec{r}_2, ..., \vec{r}_N) = \frac{1}{2} \sum_{i,j} v_{ij}(\vec{r}_i, \vec{r}_j) \tag{1}$$

reaches a minimum. Therein, $v_{ij}$ denotes the pair-potential between two particles $i$ and $j$. We denote the resulting energy of the minimum as $\epsilon_0$. If now a constant force is applied on a single particle, the system will typically not reside at the minimum. Instead, as it is depicted in Fig. 2(a), it is slightly translated along the force direction until the restoring force of the potential and the external force compensate each other. This position corresponds to a potential energy slightly higher than $\epsilon_0$ which is denoted as $\epsilon_F$.

In our article we discuss the kinetics of the system as a function of the depth of the minimum, thus, as a function of $\epsilon_0$. Since the *de facto* states of the system are given by

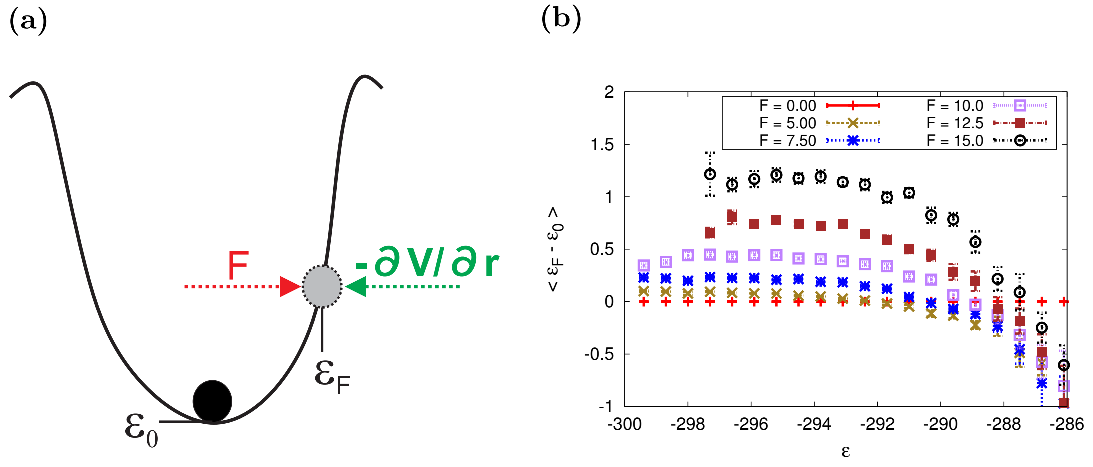


FIG. 2: **PEL under an applied external force.** (a) Schematic picture of a single PEL minimum with an external force $F$ applied. The restoring force is given by the negative gradient $-\partial V/\partial r$ parallel to the force direction. (b) Average energy difference between the original minimum $\epsilon_0$ and the resting point $\epsilon_F$ at temperature $T = 0.475$ and different forces $F$.

$\epsilon_F$, one might ask whether the nontrivial dependence of the escape kinetics on the energy is just an artificial effect due to the fact that the difference between $\epsilon_0$ and $\epsilon_F$ is dependent on the $\epsilon_0$. For this purpose we have computed the for each minimum the value of $\epsilon_F$ by minimizing $V_0 + r_\| \cdot F$, where $r_\|$ denotes the spatial coordinate of the tracer particle parallel to the direction of the external force. This computation have been conducted under the condition that the center of mass of the system is fixed. The optimized coordinates have eventually been inserted in Eq. (1) to obtain $\epsilon_F$. The average difference $\langle \epsilon_F - \epsilon_0 \rangle$ is shown in Fig. 2(b) as a function of $\epsilon_0$. As one might expect, the difference between both energies increases with increasing force in a nonlinear way, thereby indicating anharmonic character of the potential energy minimum.

It is important to notice, that typical values of $E_{\text{app}}$ are larger than unity, thus, no relaxation to other minima occurs. Furthermore, in the rage of energies $\epsilon_0 < -293$, where activated dynamics are expected, the shift displays no dependences on the depth of the minimum. Using $\epsilon_0$ therefore does not introduce an additional energy dependence to the system. Instead, it allows one to quantitatively compare observables for systems with different force strength, because the definition of $\epsilon_0$ is independent from the external force and all states belong to the very same PEL.

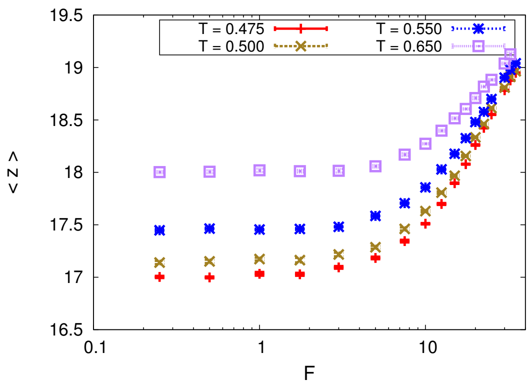


FIG. 3: **Participation number during a MB transition.** Average participation number $\langle z \rangle$ for different forces $F$ at different bath temperatures $T$.

## PARTICIPATION NUMBER IN THE FORCE DRIVEN SYSTEM

In our paper we discuss the local rates of escaping from a single minimum as a function of its potential energy $\epsilon$. One finds that the energy barrier $E_{\text{app}}$ the system has to overcome is not directly given by the depth of the metabasin (MB) $\epsilon$, like one would expect it from the standard trap model[4], but $E_{\text{app}} \propto m \cdot \epsilon$ with $m < 1$. This factor can be rationalized by considering that, even in a small simulated system, during a single process just a small fraction of particles is significantly relaxing while the others mainly remain at their positions. Formally, one can divide the system into $M$ non-interacting subsystems, each relaxing with a local escape rate $\Gamma_i(\epsilon_i)$. Assuming that the potential energy is distributed equally, one obtains for the overall relaxation rate $\Gamma_\epsilon = M\Gamma_i(\epsilon/M)$, or rather, (with $m = 1/M$) $\Gamma_\epsilon \propto \exp(m\epsilon)$.

During the connection of the local escape rates with the thermodynamic effective temperature, we assume that the factor $m$ stays constant, thus, that the number of subsystems is largely independent from the applied force. Of course, there is no geometric criterion to split the system into its constituents, however, one can measure the average number of particles which are active during a single relaxation event. As a definition for the participation number $z$ during a specific MB transition we use[5]

$$z = \sum_{i=1}^{N_{\text{A}}} \frac{\delta r_i}{\delta r_{\text{max}}}. \tag{2}$$

Therein, the sum is over all type A particles except for the tracer particle, $\delta r_i$ is the displace-

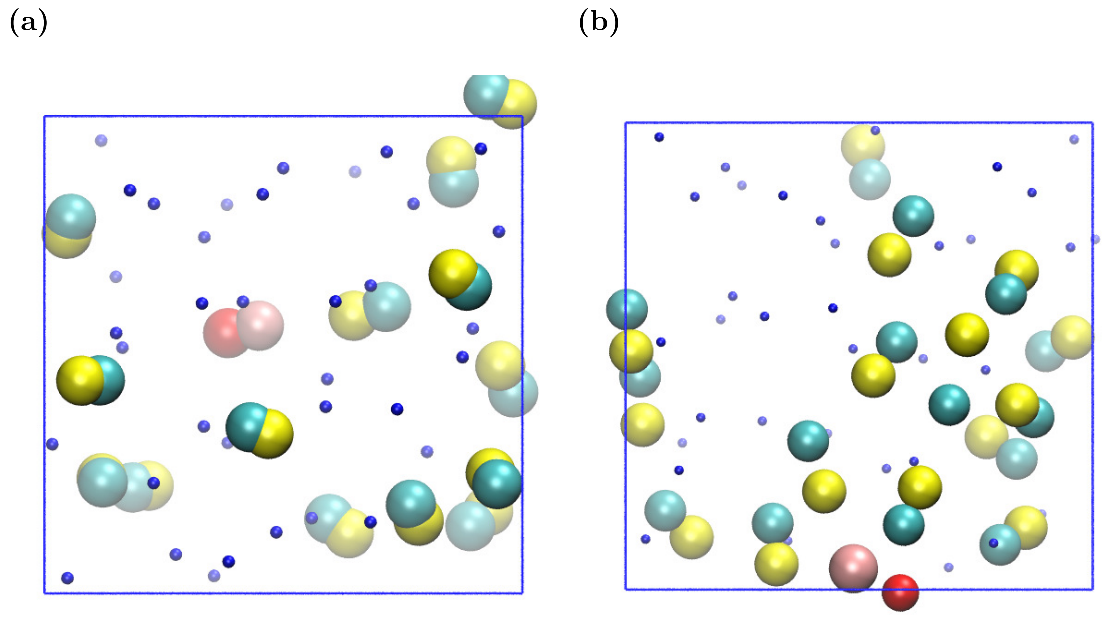

FIG. 4: **Particle motions during a single MB transition.** (a) Position of the mobile particles (see text) before and after a single MB transition at a temperature $T = 0.475$ and $F = 0$. The large colored spheres represent the mobile fraction of the particles whereas the small dark blue spheres are the immobile fraction. The positions of the bath particles before and after the transition are colored in light blue and yellow, the position of the tracer particle in brown and red, respectively. (b) The same but with a force $F = 25$. The force drags the tracer particle to the right hand side.

ment of particle $i$ and $\delta r_{\mathrm{max}}$ the maximum displacement of a particle during this particular MB transition. The value $z$ then reflects the absolute number of active particles. This definition has been successfully applied on binary mixtures[5] before. In Fig. 4, an example for the positions of the mobile particles before and after a MB transition is shown for the quiescent case (a) and for $F = 25$ (b). For the figure, a particles is defined as mobile, if it moves more than $0.5 \cdot \delta r_{\mathrm{max}}$ during this particular transition; this criterion is similar but not identical to the participation number defined in Eq. (2).

In Fig. 3, the average participation number $\langle z \rangle$ is shown at different forces $F$ and temperatures $T$. One observes that both force and temperature slightly increase the average number of involved particles. Considering, however, the scale of the ordinate, one can recognize that the effect is rather small: At the lowest temperature, the average number of active particles increases from 17 to 19 particles, thus, there is a relative increase of $\sim 10\%$.

At higher temperatures, the effect is even smaller. This observation supports the idea, that the relaxation processes are, concerning the number of involved particles, not very different from equilibrium. Treating the number of subsystems, and therefore $m$, as constant is thus a reasonable approximation.

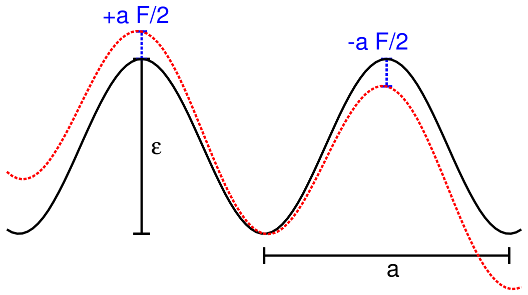


FIG. 5: **One-dimensional model PEL.** Schematic representation of a one-dimensional cosine potential. $\epsilon$ denotes the depth of the unperturbed local minima of the potential, $a$ is the distance between two of minima. If a constant force $F$ (here acting from the left to the right) is applied, the barrier along the force direction is reduced by $aF/2$. In the same manner, the barrier against the force direction is increased by the same value.

## EFFECTIVE TEMPERATURES IN A SIMPLE MODEL PEL

A central result in our main paper is the existence of an effective temperature $T_{\text{eff}}$ that controls the thermodynamic and kinetic properties of the system. This temperature turns out to be function of the squared force $F$

$$T_{\text{eff}} = T + \chi F^2, \tag{3}$$

where the parameter $\chi$ is the same for all forces and bath temperatures. For a microscopic understanding, it would be however helpful to obtain some information about the origin of this parameter, i.e., which properties of the energy landscape influence the magnitude of $\chi$.

Some insights can be obtained from evaluating the escape rates of a single particle in a tilted one-dimensional periodic cosine potential. A schematic visualization of this model can be found in Fig. 5. Without an external force, the rate of escaping from a single minimum is given by

$$\Gamma(T) = 2\Gamma_0 \, e^{-\frac{\epsilon}{T}}, \tag{4}$$

where the prefactor $\Gamma_0$ adjusts the time scale of the escape and $\epsilon$ and $T$ denote the depth of the minimum and the temperature, respectively. If the force is switched on, the potential

becomes tilted: The barrier along to the force direction is reduced by $aF/2$, where $a$ is the distance between two minima in the periodic potential, whereas the barrier against the force direction is increased by the same value. The overall escape rate in the tilted PEL results in:

$$\frac{\Gamma(F,T)}{\Gamma_0} = \left(e^{-\frac{aF}{2T}} + e^{+\frac{aF}{2T}}\right) e^{-\frac{\epsilon}{T}} = 2\cosh\left(\frac{aF}{2T}\right)\, e^{-\frac{\epsilon}{T}}. \tag{5}$$

For small $F$, the hyperbolic cosine can be expanded in a second order Taylor series and the expanded terms afterwards identified with a squared exponential function:

$$\frac{\Gamma(F,T)}{\Gamma_0} \approx 2\, \left(1 + \frac{a^2F^2}{8T^2}\right)\, e^{-\frac{\epsilon}{T}} = 2\; e^{-\frac{\epsilon}{T}+\frac{a^2F^2}{8T^2}}. \tag{6}$$

After factoring out $-\epsilon/T$ and using the approximation $1 + x \approx 1/(1-x)$ for small $x$, one can rewrite the force-dependent escape rates

$$\frac{\Gamma(F,T)}{\Gamma_0} \approx 2\; e^{-\frac{\epsilon}{T}\left(1-\frac{a^2F^2}{8\epsilon T}\right)} \approx 2\exp\left(-\frac{\epsilon}{T}\left(\frac{1}{1+\frac{a^2F^2}{8T\epsilon}}\right)\right) = \frac{\Gamma(0,T_{\text{eff}})}{\Gamma_0} \tag{7}$$

with

$$T_{\text{eff}} = T + \frac{a^2}{8\epsilon}F^2. \tag{8}$$

Here, Eq. (8) serves as a definition of an effective temperature. Within this model, a comparison of Eq. (3) and Eq. (8) allows one to relate the parameter $\chi$ with the squared distance $a^2$ between two minima and the energy barrier $\epsilon$. Both, $\epsilon$ and $a^2$ are independent from force and temperature which is in agreement with the observed properties of $\chi$. The test of this relation for the parameters of binary Lennard-Jones mixture is shown in the main article. Please note that a quantitative agreement cannot be expected, since the model potential used above is very much simpler than the PEL studied in the main article. Furthermore, Eq. (8) is valid only in the limit of small $F$ whereas Eq. (3) seems to hold even for very large forces. Nevertheless, even a power of magnitude agreement offers some insights into the microscopic origin of $\chi$, because it clarifies which properties of the energy landscape are relevant the scaling of the nonlinear response.

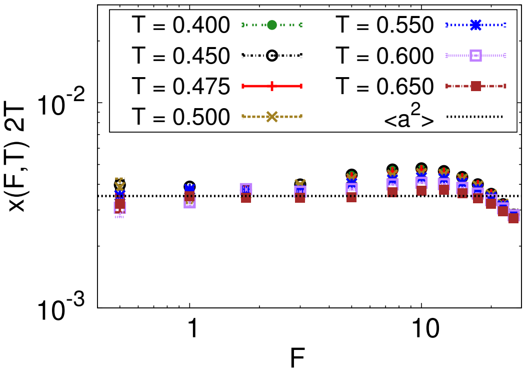


FIG. 6: **Length scale of the nonlinear mobility.** Length scale $x(F, T)$ times twice the temperature $T$ as a function of the force $F$. The black dotted line corresponds to the expectation value in the linear response regime, see Eq. (13).

## LENGTH SCALE OF THE NONLINEAR MOBILITY

In our main article, we express the nonlinear mobility $\mu$ in terms of its spatial and temporal constituents

$$\mu = x(F, T)\ \langle\Gamma(F, T)\rangle_P, \tag{9}$$

where $x(F, T)$ is the relevant length scale and $\langle\Gamma(F, T)\rangle_P$ the average hopping rate, whose properties have been broadly discussed in the main article. The dependence of $x(F, T)$ on force $F$ and temperature $T$ has already been discussed in[6]. In particular it has been shown that $x(F, T)$ displays a very weak nonlinear response and it is proportional to $1/T$ and, thus, independent from the force in the linear response regime. Since this properties become important in the present work, they shall be briefly recapitulated in the following.

Numerically, the $x(F, T)$ can be determined by dividing the average displacement $\langle\Delta x_{\|}\rangle$ of the tracer particle parallel to the force direction during a single MB transition by the force $F$:

$$x(F, T) = \langle\Delta x_{\|}\rangle / F. \tag{10}$$

In the limit of small forces, one can derive a prediction for $x(F, T)$ in the linear response regime. For this purpose, one considers the linear response relation of the mobility $\mu$

$$\mu = D/(k_{\mathrm{B}}T), \tag{11}$$

where $D$ denotes the quiescent diffusion coefficient and $k_{\mathrm{B}}$ Boltzmann constant, which is set to unity in the following. Now one can separate both the mobility and the diffusion coefficient into their spatial and temporal constituents:

$$x(F,T)\ \langle \Gamma(T)\rangle_P = (\langle a^2\rangle/2)\ \langle \Gamma(T)\rangle_P\ /T. \tag{12}$$

Here, $\langle a^2\rangle$ denotes the diffusive length scale of a type A particle, which have been found to be independent from temperature[7]. Please also notice that we have skipped the force $F$ in the argument, since, in the linear response regime, $\langle \Gamma(T)\rangle_P$ is independent from the external force. Dividing both sides of the equation by $\langle \Gamma(T)\rangle_P$ finally yields a prediction for the length scale $x(F,T)$:

$$x(F,T) = \langle a^2\rangle/(2T). \tag{13}$$

This equation is tested for different forces and temperatures in Fig. 6. In the linear response regime, the prediction is in a very good agreement for all temperatures. In the nonlinear regime, positive and negative deviations from the value occur, however, these deviations are rather low: Even for temperatures close to the glass transition the nonlinear response is less than 50% from the expected value in the linear response regime. As we show in the main article, the time scale of the nonlinear mobility varies in the same range of forces over at least one order of magnitude. One can therefore conclude that, first, the nonlinear response of the nonlinear mobility is essentially given by the nonlinear response of the temporal part of the mobility and, second, that it is reasonable to assume that $x(F,T)$ is given by the value derived in Eq. (13), even in the nonlinear regime.

## REFERENCES


[1] S. Nosé, Mol. Phys. **52**, 255 (1984).

[2] W. G. Hoover, Phys. Rev. A **31**, 1695 (1985).

[3] G. J. Martyna, M. L. Klein, and M. Tuckerman, J. Chem. Phys. **97**, 2635 (1992).

[4] C. Monthus and J.-P. Bouchaud, J. Phys. A: Math. Gen. **29**, 3847 (1996).

[5] M. Vogel, B. Doliwa, A. Heuer, and S. C. Glotzer, J. Chem. Phys. **120**, 4404 (2004).

[6] C. F. E. Schroer and A. Heuer, J. Chem. Phys. **138**, 12A518 (2013).

[7] B. Doliwa and A. Heuer, Phys. Rev. E **67**, 030501 (2003).
